# Supplementary material for: Biological Regulatory Networks are Minimally Frustrated
Source: arXiv:1911.10252 ancillary file (2019-11-22)
Supplement: Supplementary file 1 [file Supplemental_Material.pdf]

# Supplemental Material
# Biological Regulatory Networks are Minimally Frustrated

Shubham Tripathi, David A. Kessler, and Herbert Levine

## I. SUPPLEMENTAL FIGURES

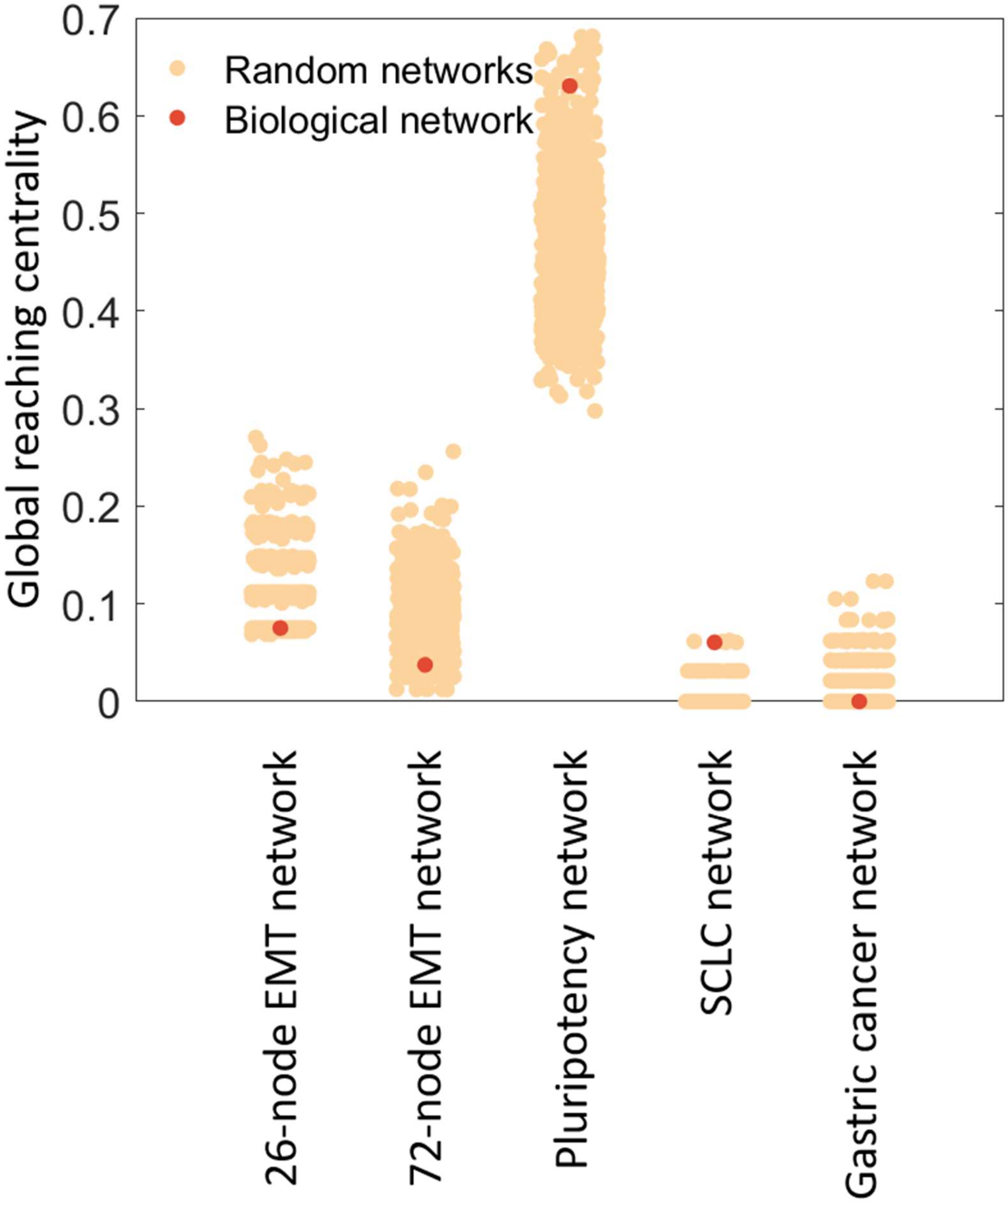


FIG. S1 Effect of randomization on hierarchy in the biological networks analyzed in the present study. Global reaching centrality [1], a measure of hierarchy in unweighted, directed networks, for the five biological networks and the corresponding random networks. While our random networks generation routine (see Supplemental Material, section II (b)) preserves various topological features including node in-degree and out-degree distributions, and the total number of activating and inhibitory interactions between network nodes, the random networks generated may be more or less hierarchical than the corresponding biological network. Our analysis reveals that in either case, biological networks are minimally frustrated as compared to their random counterparts.

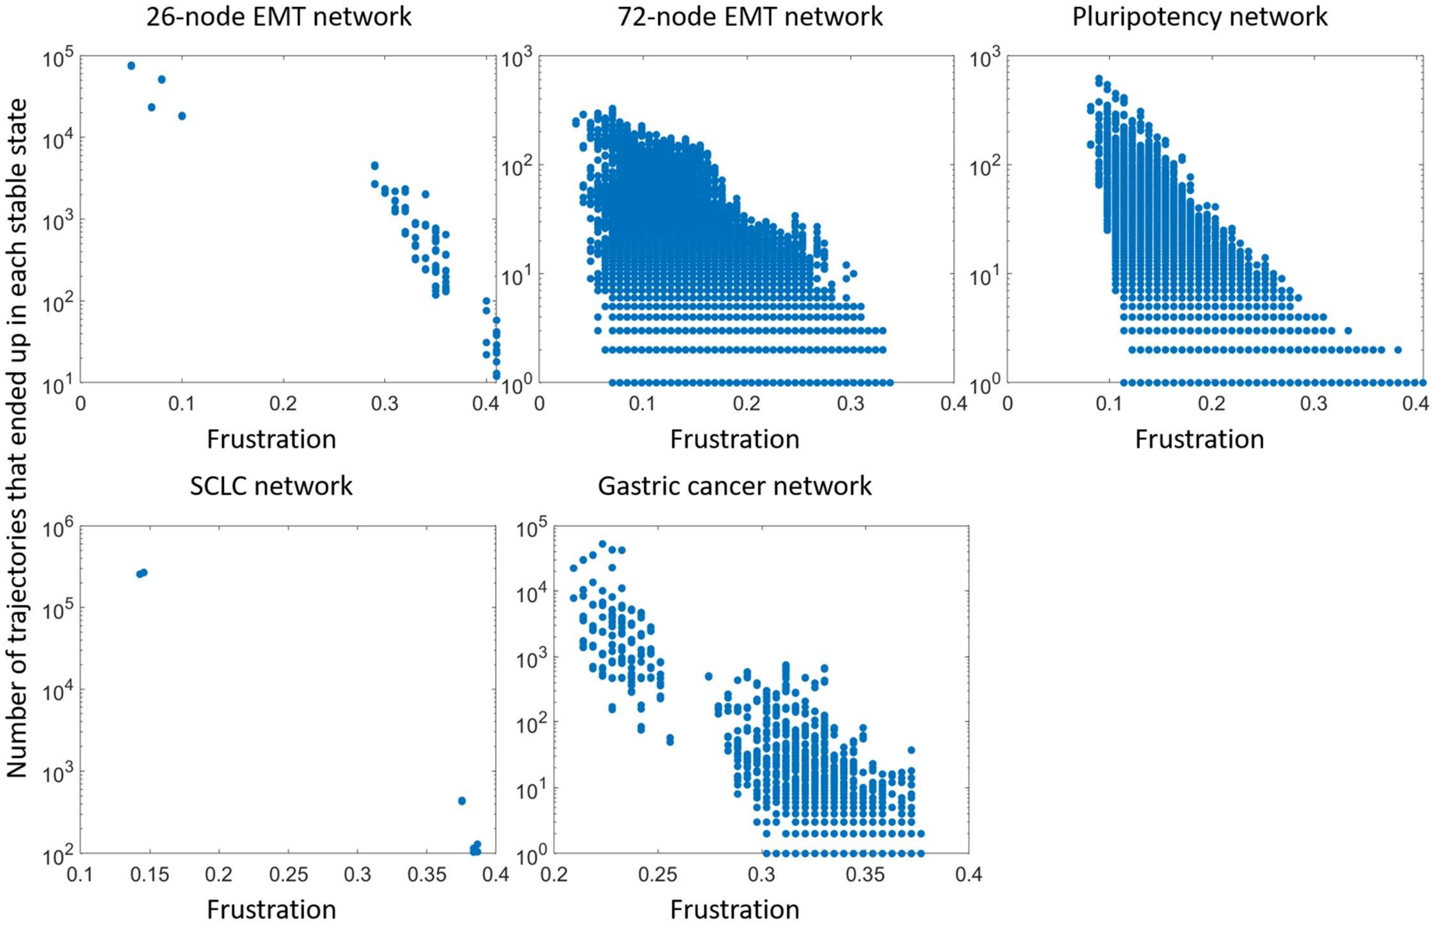


FIG. S2 Correlation between the frustration of a stable state and how frequently it is encountered when simulating network dynamics starting from random initial conditions. In the case of each biological network, low frustration stable states are more likely to be reached as compared to high frustration stable states.

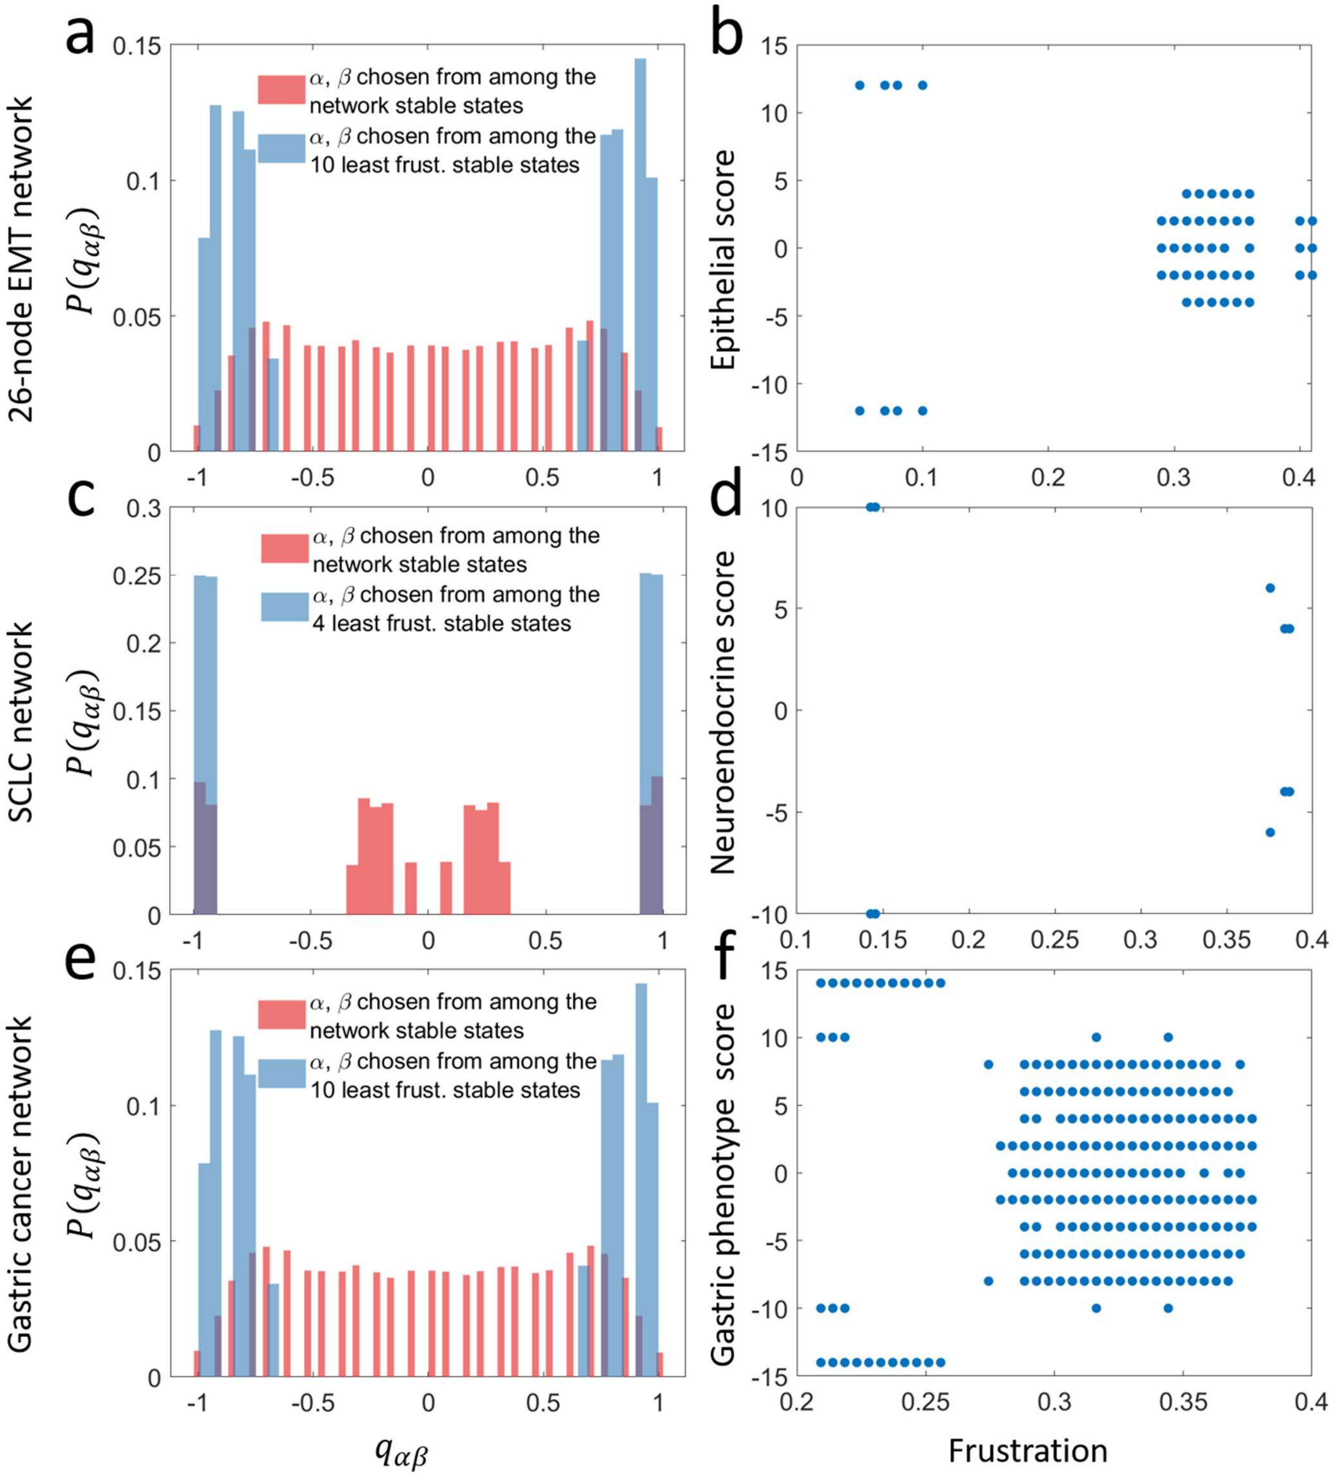


FIG. S3 Minimally frustrated stable states of biological networks define canonical cell types. (a), (c), (e) $P(q_{\alpha\beta})$ is bimodal for the minimally frustrated stable states of the 26-node EMT network (a), the SCLC network (c), and of the gastric cancer network (e). (b), (d), (f) Gene expression patterns in minimally frustrated stable states of the three biological networks correspond to canonical cell types. In (b), a high, positive score indicates an epithelial phenotype while a low, negative score indicates a mesenchymal phenotype. In (d), a high, positive score indicates a neuroendocrine phenotype while a low, negative score indicates a mesenchymal phenotype. In (f), a high, positive score indicates a gastric phenotype while a low, negative score indicates an intestinal phenotype. In all three scenarios, high frustration stable states represent ambiguous cell fate choices.

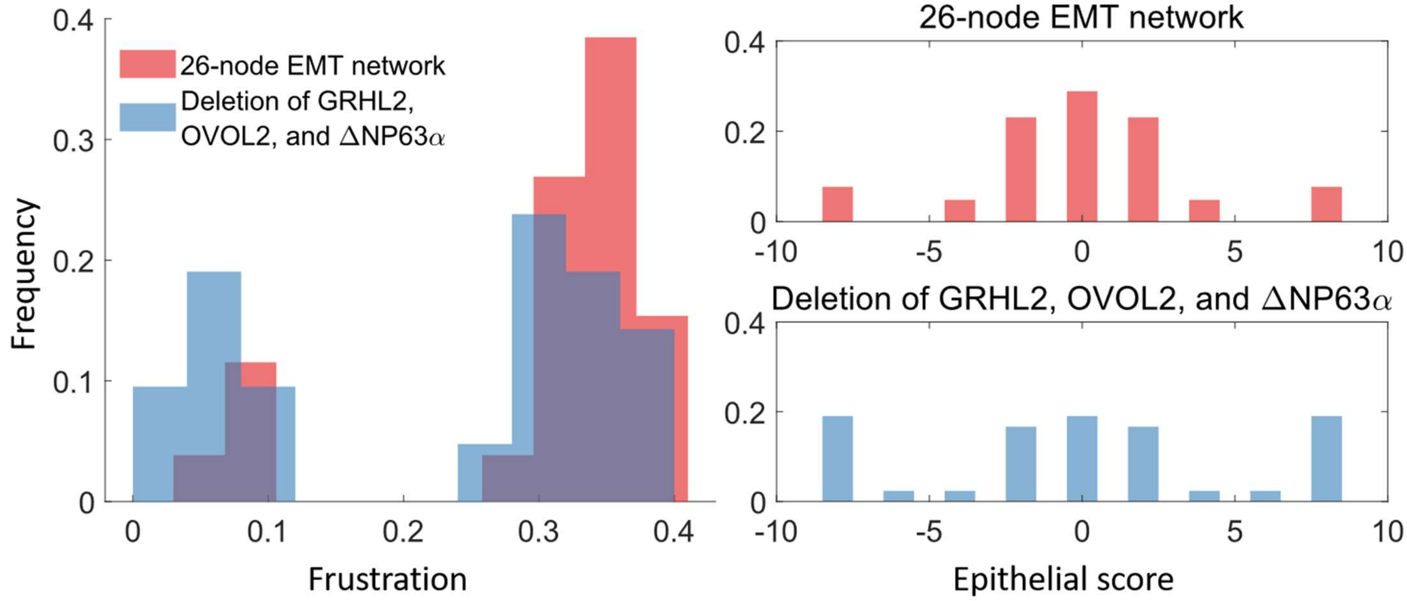


FIG. S4 Effect of deletion of factors known to stabilize phenotypic states with co-expression of epithelial and mesenchymal markers. Experimental studies have shown that the three factors, GRHL2, OVOL2, and ΔNP63$\alpha$ can stabilize cells that co-express both epithelial and mesenchymal markers (indicated by an intermediate value of the epithelial score in our framework). (Left panel) Deletion of these three factors from the 26-node EMT network led to stable states with lower frustration and (Right panel) decreased the fraction of stable states with intermediate values of the epithelial score.

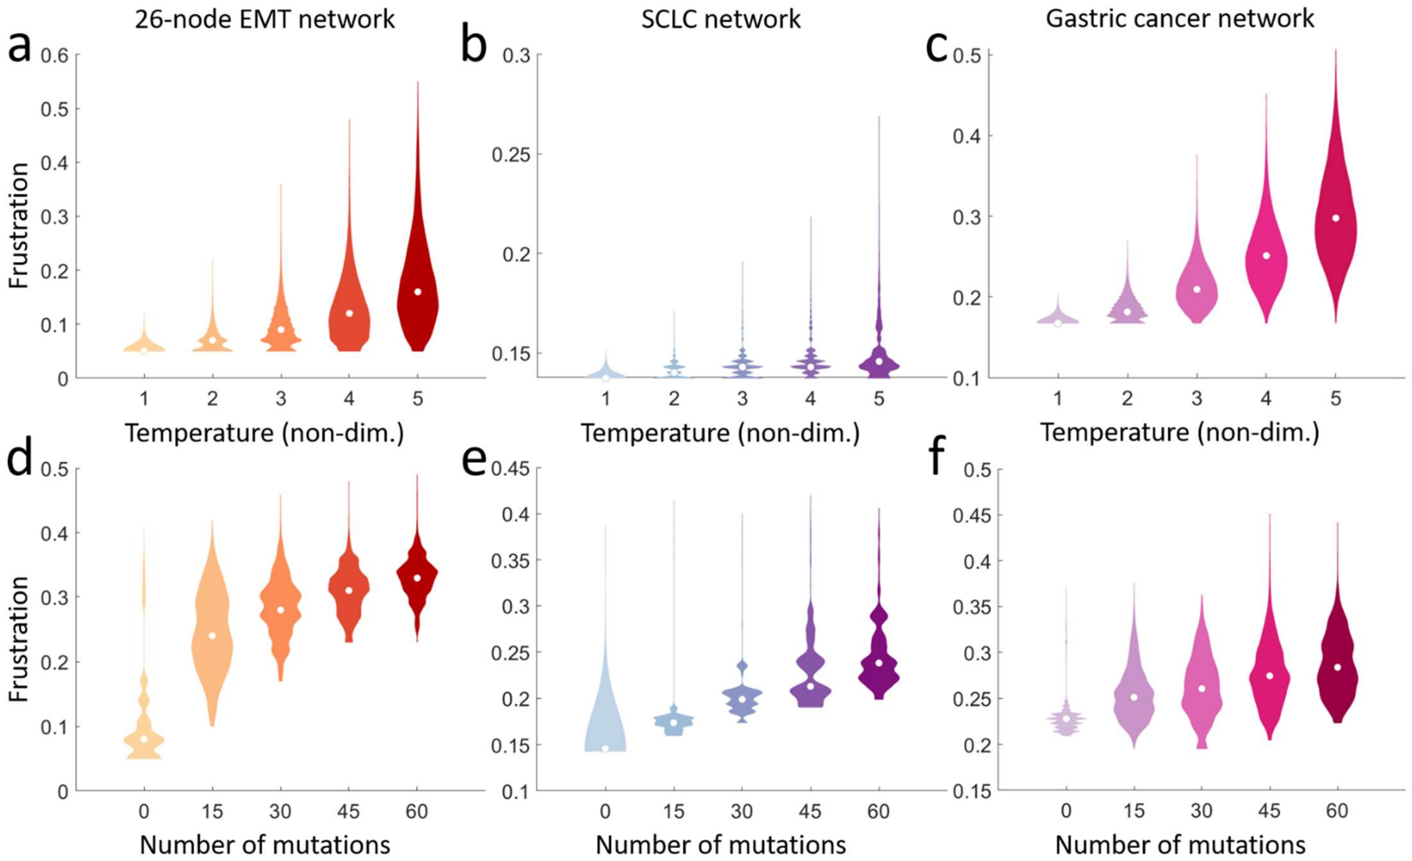


FIG. S5 High frustration stable states are increasingly occupied under noisy dynamics or if the biological network accumulates mutations. (a)-(c) Frustration of the observed network states at non-zero pseudo-temperatures, i.e., under noisy node dynamics. The dynamics become more and more noisy as the pseudo-temperature is increased. (d)-(f) Frustration of the observed network states when mutations are introduced into biological networks (without noisy dynamics). The white circle in each violin indicates the median.

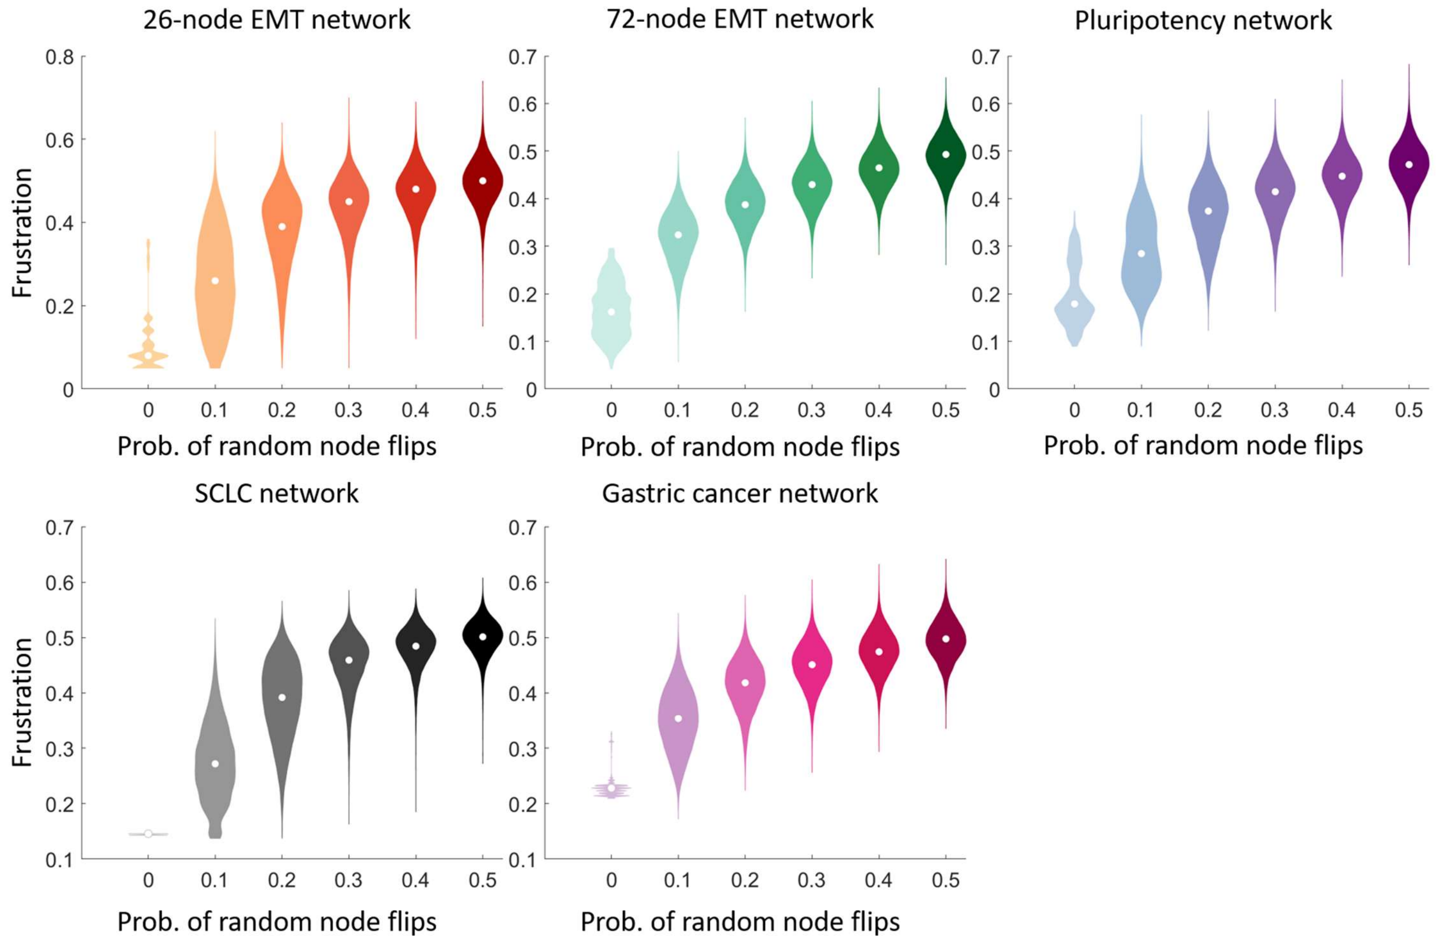


FIG. S6 An alternate approach to probing network behavior under noisy dynamics. In this setup, after updating the value of a network node using Eq. (1), its value is flipped with a certain probability. The plots show the frustration of the observed network states for different probabilities of random node flips. The white circle in each violin indicates the median.

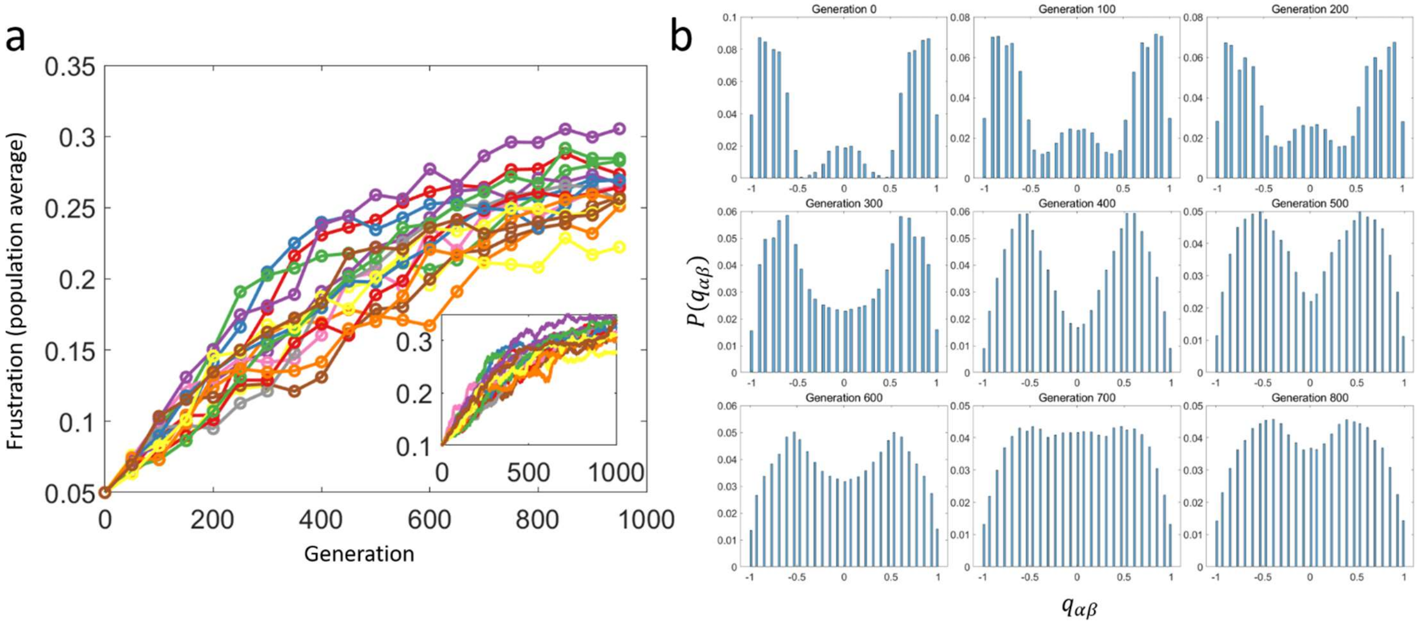


FIG. S7 Onset of generic random network behavior with the accumulation of mutations in networks in a population. We simulated the dynamics of a population of networks in the absence of selection but in the presence of mutation. Starting with a population of 500 identical networks (identical to the 26-node EMT network), each subsequent generation was populated by randomly choosing networks from the previous generation with equal probability and mutating each network with a probability of 5%. The mutation step involved randomly choosing a pair of network edges and switching their target nodes. (a) Frustration of the least frustrated observed network state averaged over the networks in the population. Different colors indicate independent simulation runs. The inset shows the state frustration averaged over the end state of simulations starting from 50 random initial conditions for each network followed by averaging over the networks in the population. (b) $P(q_{\alpha\beta})$ at different time points during the simulation, shown for one of the simulation runs. The distribution becomes less and less bimodal as the simulation proceeds.

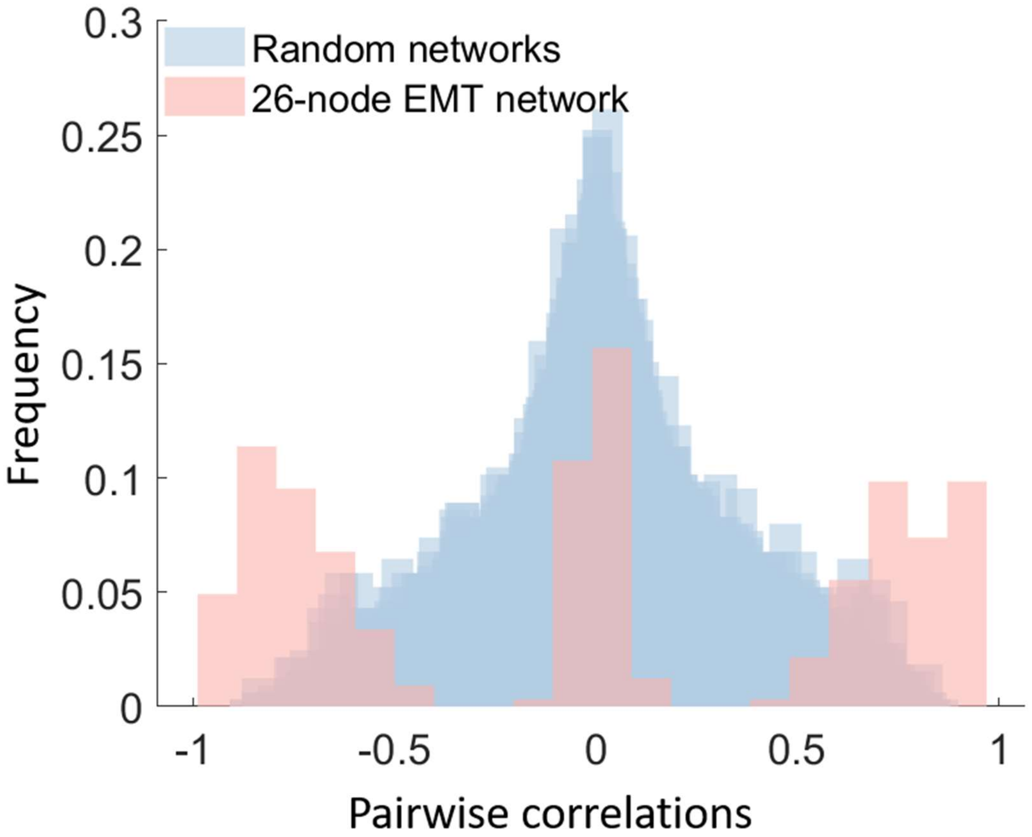


FIG. S8 Differences between the stable steady states of a biological network and those of random networks in an ordinary differential equations-based modeling framework. We used the random circuit perturbation technique to determine the stable steady states of the 26-node EMT network and of random networks with similar topological features (see Supplemental Material, section II (g)). The distribution of correlations between network nodes calculated across stable steady states is tri-modal for the 26-node EMT network— expression levels of some node pairs are strongly positively correlated, expression levels of some node pairs are strongly negatively correlated, and expression levels of some nodes pairs are uncorrelated. In contrast, pairwise correlations across stable states of random networks are clustered around 0. In the main text, we have shown that the existence of minimally frustrated stable states distinguishes biological networks from random networks in the context of a Boolean modeling framework. This figure indicates that the existence of tri-modally distributed pairwise correlations across stable steady states may distinguish biological networks from random networks in an ordinary differential equations-based modeling framework.

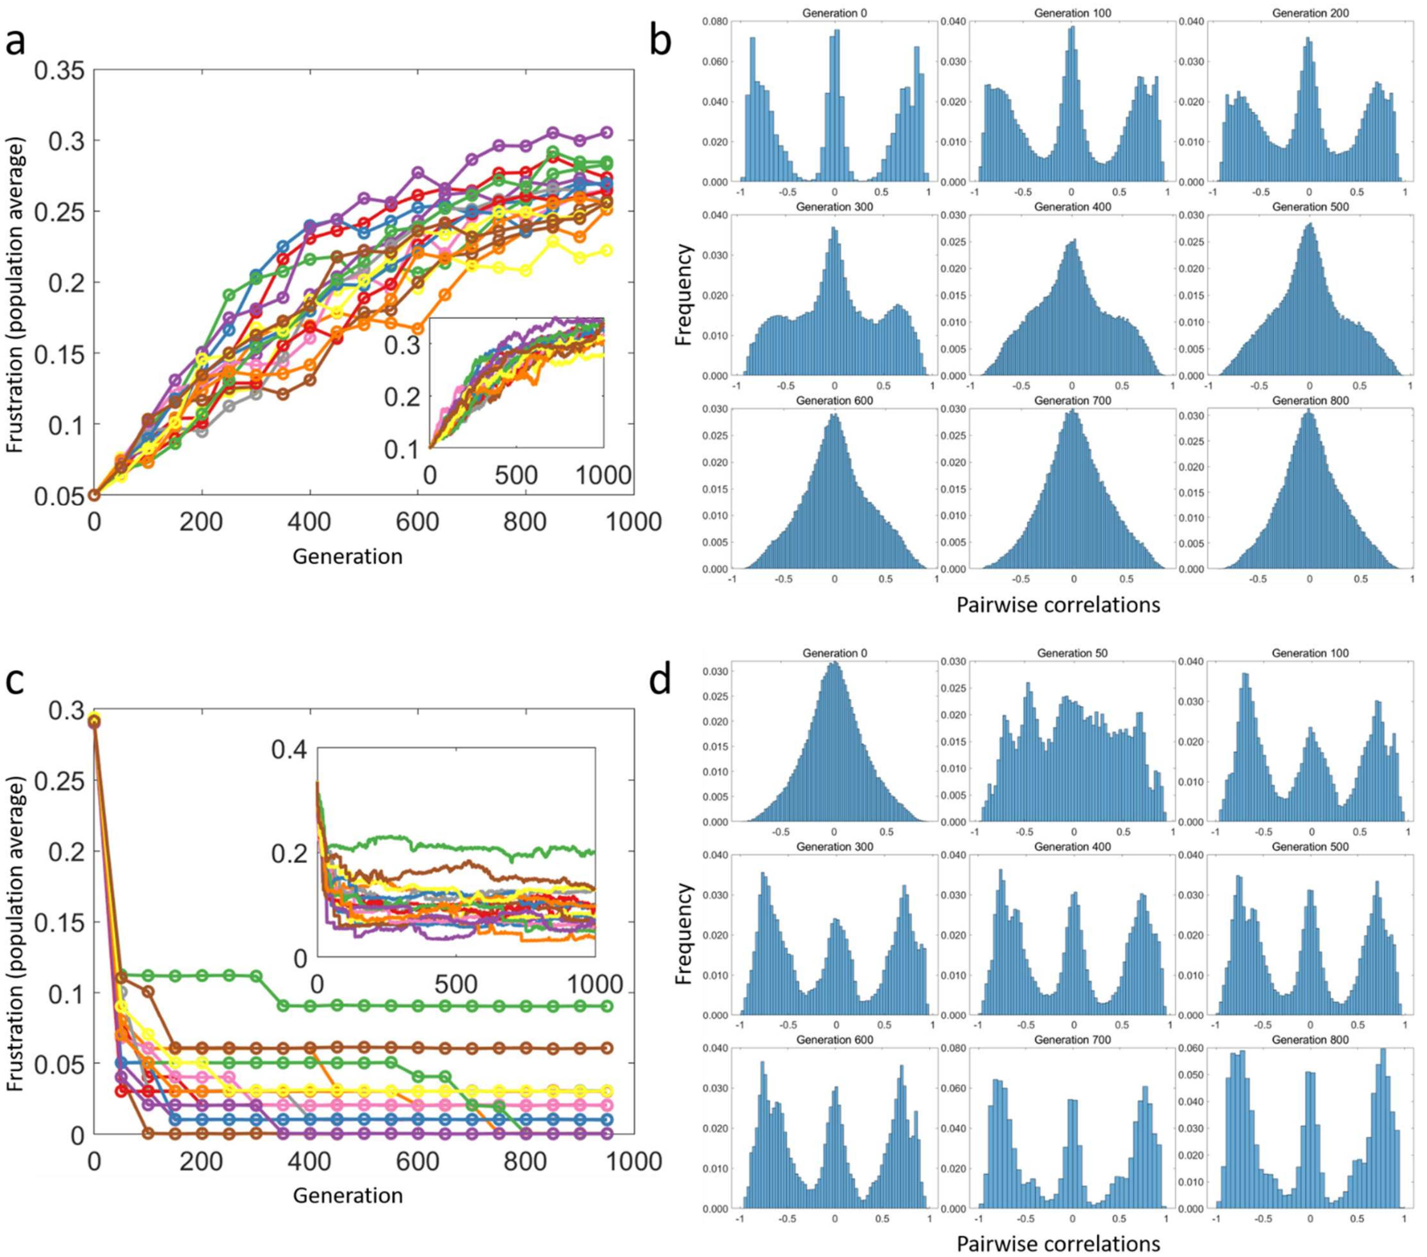


FIG. S9 Implications of frustration of the stable states of networks in a population for network behavior in an ordinary differential equations-based modeling framework. (a) Same as Fig. S7 (a) which illustrates the increase in frustration of observed states as networks in the population accumulate mutations. (b) Distribution of pairwise correlations across stable steady states of networks in the population at different time points during the simulation. We used random circuit perturbation (see Supplemental Material, section II (g)) to determine the stable steady states of networks in the population at different points. As the simulation proceeds, the distribution of pairwise correlations loses tri-modality (a property of biological networks; Fig. S8) and becomes clustered around 0 (same as the distribution of pairwise correlations for random networks; Fig. S8). (c) Same as Fig. 4 (Top) which illustrates the evolution of biological behavior by a population of random networks under selection for networks with low frustration states. (d) Distribution of pairwise correlations across stable steady states of networks in the population at different time points during the simulation. Stable steady states of networks in the population were determined using random circuit perturbation (see Supplemental Material, section II (g)). As the simulation proceeds, pairwise correlations across stable steady states go from being clustered around 0 (a property of random networks; Fig. S8) to being tri-modally distributed (a property of biological networks; Fig. S8).

## II. METHODS

*(a) Biological networks chosen for analysis.*— The 26-node epithelial-mesenchymal transition (EMT) network [2] has been proposed to regulate transitions between epithelial and mesenchymal phenotypic states in cells. The 72-node EMT network [3] has been used to investigate epithelial-mesenchymal transition and mesenchymal-epithelial transition in hepatocellular carcinoma [4,5]. The pluripotency network [6] has been constructed by manually collecting evidence from the literature and includes the major regulatory interactions that are known to operate in human embryonic stem cells. The small cell lung cancer (SCLC) network [7] was constructed using gene expression data from cancer cell lines and using manual literature search. The network was then used to describe the small cell lung cancer-associated phenotypes— neuroendocrine and mesenchymal. Finally, the gastric cancer network [8] was also constructed using data from the literature and has been used to describe transitions between gastric and intestinal phenotypic states in gastric cancer cells.

*(b) Generation of random networks.*— Random networks corresponding to each biological network were generated using a procedure that preserved certain topological features of the biological network— a pair of edges in the biological network were randomly chosen and their target nodes were switched; this operation was repeated multiple times to obtain a random network. In the random network thus generated, each node had the same in-degree and the same out-degree as the biological network. Further, the random network had the same number of activating and inhibitory interactions as the biological network. In fact, the number of nodes that a given network node activates and the number of nodes that a given network node inhibits was the same in random networks as in the corresponding biological network.

*(c) Determination of stable states of biological and random networks.*— Starting from a random initial condition, the discrete-time network dynamics were simulated using Eq. (1) for 5000 time steps. The network state at the end of the simulation run was then checked for being a stable state. For each network, biological or random, we simulated the network dynamics starting from $2^{20}$ random initial conditions to obtain the collection of stable states for the network. For the biological 26-node EMT network and 33-node SCLC network, we found all the stable states by exhaustively testing all possible states for stability. We obtained 104 stable states for the 26-node EMT network and 10 stable states for the SCLC network.

*(d) Calculation of phenotypic scores.*— For each biological network, we used the literature to determine network nodes whose expression characterizes different phenotypic states. In the case of the two EMT networks, we obtained a set of epithelial nodes and a set of mesenchymal nodes. To obtain the epithelial score for a given network state, we added $+1$ to the score for each epithelial node that had a value $+1$; we added $-1$ if an epithelial node had a value $-1$. We also added $+1$ to the score for each mesenchymal node that had a value $-1$ and added $-1$ if a mesenchymal node had a value $+1$. To calculate a stemness score for states of the pluripotency network, we used the set of pluripotency markers and the set of differentiation markers defined previously [6]. Neuroendocrine scores for the states of the SCLC network and gastric phenotype scores for the states of the gastric cancer network were similarly calculated. Node sets used for phenotypic score calculation in each case are listed in Table S1.

*(e) Simulation of noisy network dynamics.*— We used the finite-temperature Metropolis Monte Carlo algorithm [9,10] to simulate noisy network dynamics. Briefly, the state of a randomly chosen network node was flipped. If the flip decreased the value of the pseudo-Hamiltonian, the flipping move was accepted, and the network state was updated accordingly. If the flipping move increased the value of the pseudo-Hamiltonian, the move was accepted with a probability $e^{-(\frac{\Delta H}{T})}$ where $\Delta H$ is the change in the value of the pseudo-Hamiltonian upon flipping the randomly chosen node and $T$ is the non-dimensionalized pseudo-temperature. If the flipping move was rejected, the network state was kept unchanged. The network dynamics thus become increasingly noisy as the pseudo-temperature is increased since flipping moves that increase the value of the pseudo-Hamiltonian are more likely to be accepted at higher temperatures.

The procedure described above was repeated $N$ times where $N$ is the number of nodes in the network. This constituted 1 Monte Carlo step. We simulated network dynamics at a given temperature for 5000 Monte Carlo steps. After discarding the simulation results for the first 2500 Monte Carlo steps, we reported the network state

every 50 steps. For each network, 16 independent runs were carried out at each pseudo-temperature to obtain the distributions shown in Fig. 3 (a), 3 (c), 3 (e), 3 (g), and S5 (a)-(c).

*(f) Simulation of evolution of biological behavior in random networks.*— By repeatedly applying the random network generation procedure to the 26-node EMT network, we obtained a population of 500 random networks. For each network in the population, we simulated the dynamics using Eq. (1) starting from 50 random initial conditions (5000 simulation steps for each random initial condition). The frustration of the network state at the end of these runs was saved. We then ranked the networks in the population in the order of the frustration of the least frustrated state recorded. The top 5% of the networks (i.e., the top 25 networks with the least frustrated observed states) were used to populate the next generation. To populate the $n^{th}$ generation, a network was randomly chosen from among the top 5% of the networks in the $(n-1)^{th}$ generation and mutated with a probability of 5%. This procedure was repeated 500 times to preserve the population size across generations. The mutation step involved randomly choosing a pair of network edges and switching their target nodes.

*(g) Determination of stable steady states of a network in an ordinary-differential equations based modeling framework.*— In Fig. S8, and in Fig. S9 (b) and S9 (d), we used the random circuit perturbation [11] technique to determine the collection of stable steady states a network can exhibit. Briefly, given a network topology, the random circuit perturbation technique generates an ensemble of kinetic models. Each model in such an ensemble has the same topology but differs from other models in the ensemble in the kinetic parameters regulating interactions between network nodes. The dynamics of each kinetic model are then simulated starting from random initial conditions using ordinary differential equations to obtain the set of stable steady states the network can exhibit.

*(i) Code availability*— The computer codes which were used to carry out the simulations reported in this study and the biological network definitions are available online on GitHub (https://github.com/st35/frustration-biological-networks).


[1] E. Mones, L. Vicsek, and T. Vicsek, PLoS One **7**, e33799 (2012).

[2] D. Jia, J. T. George, S. C. Tripathi, D. L. Kundnani, M. Lu, S. M. Hanash, J. N. Onuchic, M. K. Jolly, and H. Levine, Phys. Biol. **16**, 025002 (2019).

[3] F. Font-Clos, S. Zapperi, and C. A. M. La Porta, Proc. Natl. Acad. Sci. **115**, 5902 (2018).

[4] S. N. Steinway, J. G. T. Zanudo, W. Ding, C. B. Rountree, D. J. Feith, T. P. Loughran, and R. Albert, Cancer Res. **74**, 5963 (2014).

[5] S. N. Steinway, J. G. T. Zañudo, P. J. Michel, D. J. Feith, T. P. Loughran, and R. Albert, NPJ Syst. Biol. Appl. **1**, 15014 (2015).

[6] R. Chang, R. Shoemaker, and W. Wang, PLoS Comput. Biol. **7**, e1002300 (2011).

[7] A. R. Udyavar, D. J. Wooten, M. Hoeksema, M. Bansal, A. Califano, L. Estrada, S. Schnell, J. M. Irish, P. P. Massion, and V. Quaranta, Cancer Res. **77**, 1063 (2017).

[8] S. Li, X. Zhu, B. Liu, G. Wang, and P. Ao, Oncotarget **6**, 13607 (2015).

[9] N. Metropolis, A. W. Rosenbluth, M. N. Rosenbluth, A. H. Teller, and E. Teller, J. Chem. Phys. **21**, 1087 (1953).

[10] W. K. Hastings, Biometrika **57**, 97 (1970).

[11] B. Huang, M. Lu, D. Jia, E. Ben-Jacob, H. Levine, and J. N. Onuchic, PLoS Comput. Biol. **13**, e1005456 (2017).

# III. SUPPLEMENTAL TABLES

**Table S1 Sets of nodes used to calculate phenotypic scores for states of different networks**

| | | |
|---|---|---|
| 26-node EMT network | Epithelial nodes | CDH1, GRHL2, OVOL2, miR-200b, miR-200c, miR-34a |
| | Mesenchymal nodes | VIM, ZEB1, ZEB2, FOXC2, SNAI1, TWIST1 |
| 72-node EMT network | Epithelial nodes | Ecadherin, KLF4, cateninmemb, miR200, GSK3, TrCP |
| | Mesenchymal nodes | cateninnuc, ZEB1, SNAI1, TWIST1, ZEB2, FOXC2 |
| Pluripotency network | Stemness nodes | OCT4, SOX2, NANOG, Oct4-Sox2, KLF4, FOXD3, ZIC3, ZFP42, GDF3, TDGF1, PBX1 |
| | Differentiation nodes | FOXA2, AFP, SOX17, GATA4, GATA6, T, GATA2, GATA3, hCGa, hCGb, CDX2 |
| SCLC network | Neuroendocrine nodes | FOXA2, OVOL2, SOX2, ASCL1, LEF1 |
| | Mesenchymal nodes | SMAD3, MYC, NFKB1, ZEB1, MITF |
| Gastric cancer network | Gastric phenotype nodes | RB, GSK3B, P27, PTEN, E-cadherin, BAD, IKB |
| | Intestinal phenotype nodes | CDK46, CDK2, CMYC, beta-catenin, NFKB, ERK, JNK |
| EMT networks in Fig. S4 | Epithelial nodes | CDH1, miR-200b, miR-200c, miR-34a |
| | Mesenchymal nodes | VIM, ZEB1, SNAI1, TWIST1 |
